# Supplementary material for: OSDP: Optimal Sharded Data Parallel for Distributed Deep Learning
Source: arXiv:2209.13258 source file (2023-05-19)
Supplement: Supplementary file 1 [file appendix.tex]

% \appendix
\section{Examples of the optimal execution plans given by OSDP}
\begin{figure*}[!t]
\centering
\includegraphics[width=1\linewidth]{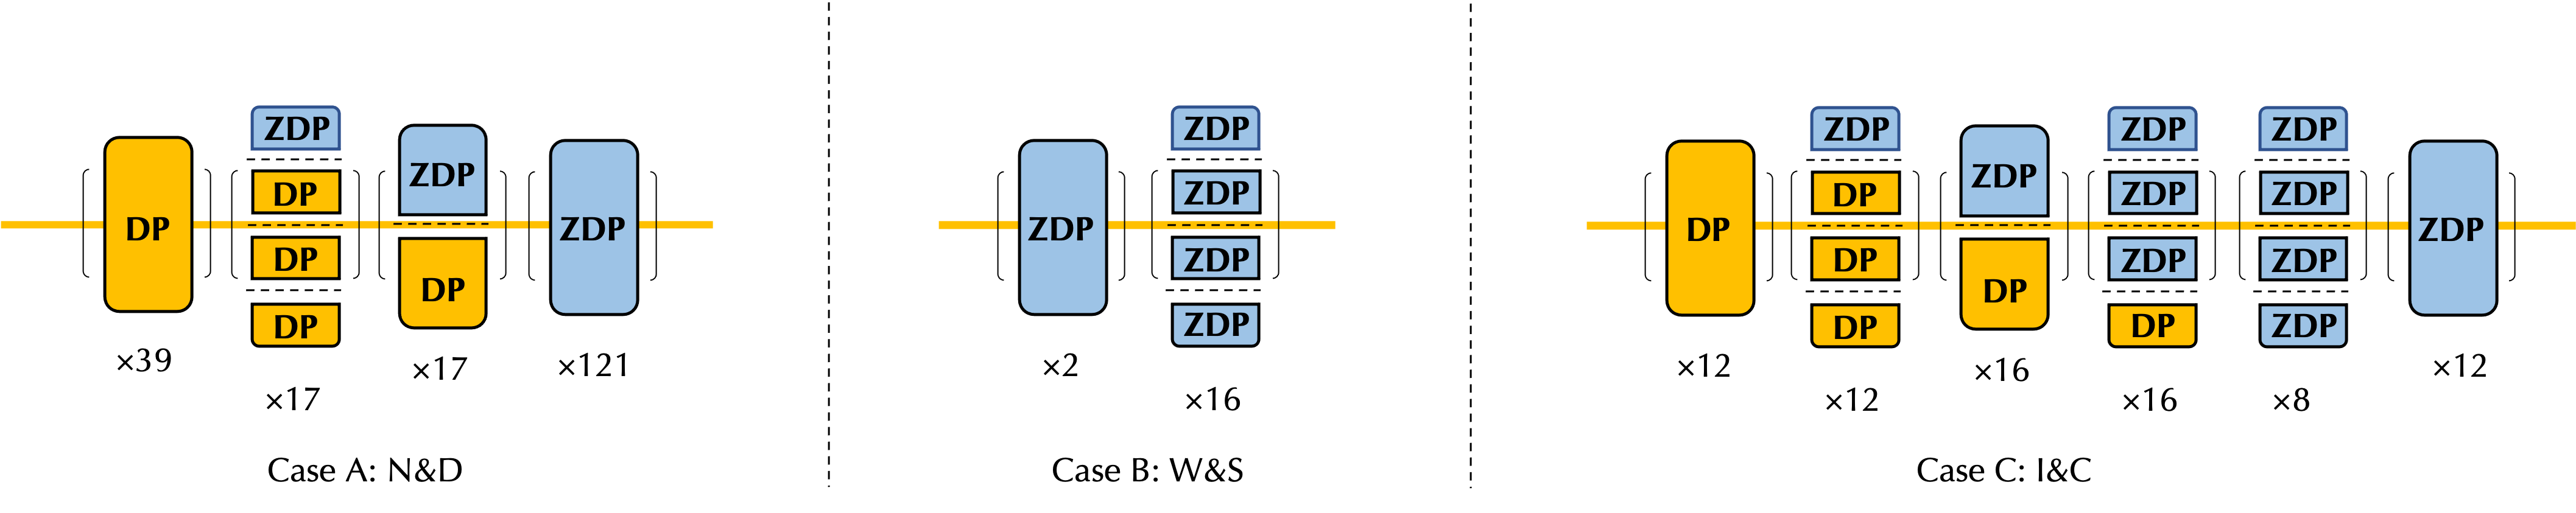}
\caption{Examples of the optimal execution plans given by OSDP for N\&D, W\&S and I\&C on 8 GPUs. Different colors represent different modes, each rectangle within each bracket donotes an operator, the split of rectangle represents the application of operator splitting. The number ×N under the rectangle means N operators are applied with this strategy.}
\label{fig:example_ex}
\end{figure*}
